# Supplementary material for: Prompt Combines Paraphrase: Teaching Pre-trained Models to Understand Rare Biomedical Words
Source: arXiv:2209.06453 source file (2022-09-14)
Supplement: Supplementary file 1 [file x.Appendix.tex]

\appendix
\section*{Appendix}

\section{Pre-trained Corpora of the Model}
\label{apendix-corpora}
We use a biomedical and clinical RoBERTa-Large \citep{lewis2020pretrained} trained on biomedical corpora, .

\section{Word Labels for Rare Biomedical Words}
\label{full-list}
We focus on the rare words which have been tagged with labels that contain any of following medicine-related strings:

['medical', 'medicine', 'disease', 'symptom', 'pharma']

\section{Dataset}
\label{appendix-stat}
We conduct our experiments on MedNLI and MedSTS datasets. Specifically, we use the available sub-datasets ClinicalSTS-2018 and ClinicalSTS-2019 for MedSTS provided by the maintainer of MedSTS project. The statistics of involved datasets can be found in Table \ref{data_stat}. Note that there is no development set split in MedSTS. Therefore, we sample the development set for MedSTS from its training set with the same quantity as sampled few-shot training set and make sure there is no overlap between training and development set.

\section{Prompt Settings}
\label{prompt-settings}
We adopt the prompt settings empirically from \citet{schick2021exploiting} and \citet{gao-etal-2021-making} for the natural language inference and semantic textual similarity tasks shown in Table \ref{prompt} since the prompt paradigm is not the core of this work and our method is prompt-agnostic.

\section{Train with More Samples}
\label{appendix-more-samples}
Besides few-shot scenarios, we also train with more samples for MedNLI since it has 11,232 training samples. Experiment results are shown in Table \ref{mednli-more}.

\section{Case Analysis}
\label{appendix-case}
We display several cases in which model predicts differently with or without paraphrases of rare biomedical words from MedNLI in Table \ref{case-study}. From the cases, we can see that paraphrases of rare biomedical words that are determinant in sentence understanding can be helpful to pre-trained model while paraphrases of those irrelevant rare biomedical words may confuse the model.
